# Supplementary material for: It's an Alignment, Not a Trade-off: Revisiting Bias and Variance in Deep Models
Source: arXiv:2310.09250 source file (2023-10-13)
Supplement: Supplementary file 1 [file appendix.tex]

\section{More results on }
